# Supplementary material for: Learning protein sequence embeddings using information from structure
Source: arXiv:1902.08661 source file (2019-10-16)
Supplement: Supplementary file 1 [file table_appendix_hyper_sensitivity.tex]

% non-extended bold font

\begin{tabular}{llllll}

\toprule

\multicolumn{1}{l}{\bf{Model}} &
    \multicolumn{1}{c}{\bf{Accuracy}} &
    \multicolumn{1}{c}{\bf{$r$}} &
    \multicolumn{1}{c}{\bf{$\rho$}} \\

\midrule

no contact prediction, no LM, no resampling & 0.88817 &	0.77671 &	0.62484 \\
no contact prediction, no LM & 0.89847 &	0.81459 &	0.64693 \\
no contact prediction, no resampling & 0.92864 &	0.85175 &	0.65897 \\
no contact prediction & 0.93794 &	0.88048 &	0.67645 \\

\hdashline
$\lambda=0.5$ & 0.9404 &	0.88566 &	0.67688 \\
$\lambda=0.33$ & 0.94358 &	0.89832 &	0.68142 \\
$\lambda=0.1$ & 0.95149 &	0.90954 &	0.69018 \\

\bottomrule

\end{tabular}
